# Supplementary material for: Wavefunction-Based Analysis of Dynamics Versus Yield of Free Triplets in Intramolecular Singlet Fission
Source: arXiv:2011.05434 source file (2020-11-10)
Supplement: Supplementary file 1 [file SuppInfo_Mazumdar-resubmit.pdf]

# Wavefunction-Based Analysis of Dynamics Versus Yield of Free Triplets in Intramolecular Singlet Fission

## Supporting Information

Rafi Chesler
*Department of Physics, University of Arizona Tucson, AZ 85721*

Souratosh Khan
*School of Information, University of Arizona Tucson, AZ 85721*

Sumit Mazumdar
*Department of Physics, University of Arizona*
*Department of Chemistry and Biochemistry, University of Arizona and*
*College of Optical Sciences, University of Arizona*
(Dated: October 29, 2020)

## A. PENTACENE DIMERS PREVIOUSLY STUDIED THEORETICALLY

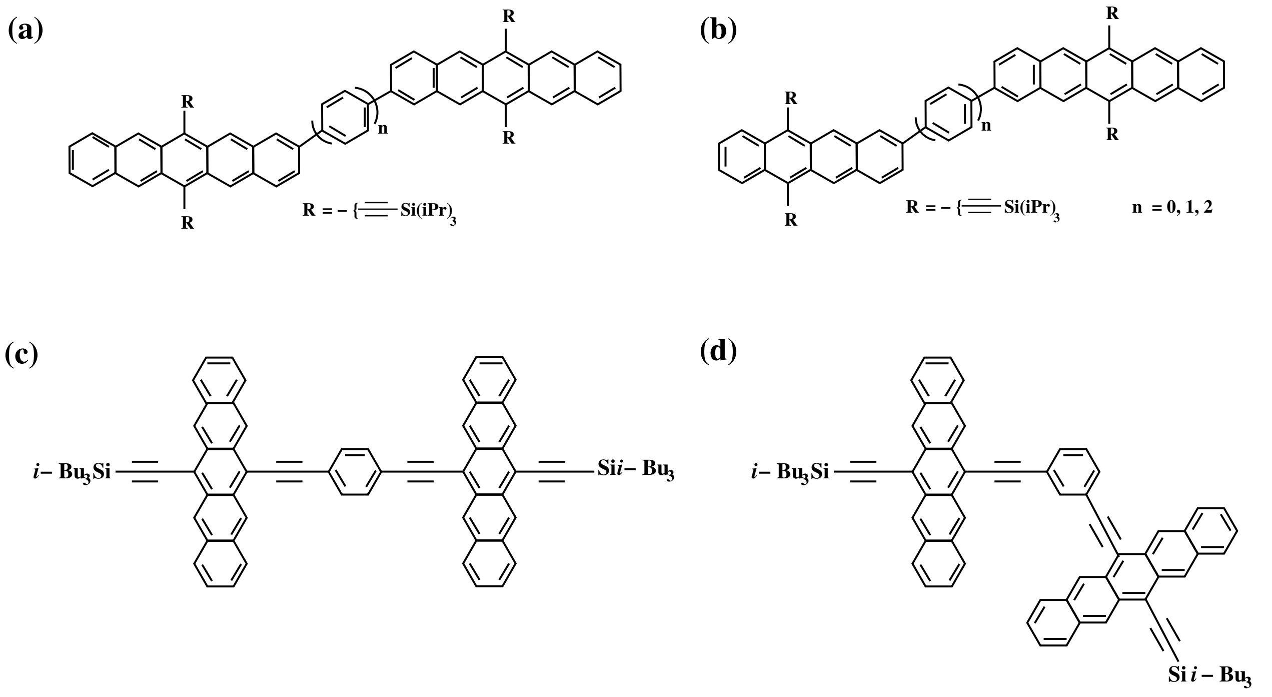


FIG. S1: TIPS-acene dimers linked via phenylene spacer groups: (a) bipentacenes BPn, (b) asymmetric pentacene-tetracene dimers PTn, and (c, d) *para*- and *meta*-(bisethynylpentacenyl)benzene dimers, *p*-Pc2 and *m*-Pc2.

## B. MONOMER CALCULATION RESULTS

TABLE S1: Experimental and calculated energies of $S_1$ and $T_1$ in anthracene, in eV.

| State | Expt | $U = 7.7$ eV $\kappa = 1.3$ |
|---|---|---|
| $S_1$ | 3.25[a] | 3.28 |
| $T_1$ | 1.82[b] | 1.67 |

[a] Pope, M.; Swenberg, C. E. *Electronic Processes in Organic Crystals and Polymers 2nd Ed.*; Oxford University Press: Oxford, U.K, 1999

[b] Lewis, G. N.; Kasha, M. Phosphorescence and the Triplet State. *J. Chem. Phys.*, **1964**, *66*, 2100-2116

## C. MULTIPLE REFERENCE SINGLES AND DOUBLES CONFIGURATION INTERACTION (MRSDCI)

TABLE S2: $N_{ref}$ and $N_{total}$ in the different subspaces of the singlet and triplet manifolds in $p-2$ and $m-2$ dimers.

| State | $p-2$ | | $m-2$ | |
|---|---|---|---|---|
| | $N_{ref}$ | $N_{total}$ | $N_{ref}$ | $N_{total}$ |
| $S_0S_0$ | 159 | 2097476 | 241 | 3998642 |
| $S_0S_1$ | 159 | 2097476 | 241 | 3998642 |
| $S_0T_1$ | 50 | 2475030 | 68 | 3490652 |
| $^1TT$ | 248 | 3558744 | 160 | 2926344 |
| $^5TT$ | 49 | 2280803 | 52 | 2369169 |

## D. WAVEFUNCTIONS OF PENTACENE DIMERS PREVIOUSLY STUDIED THEORETICALLY

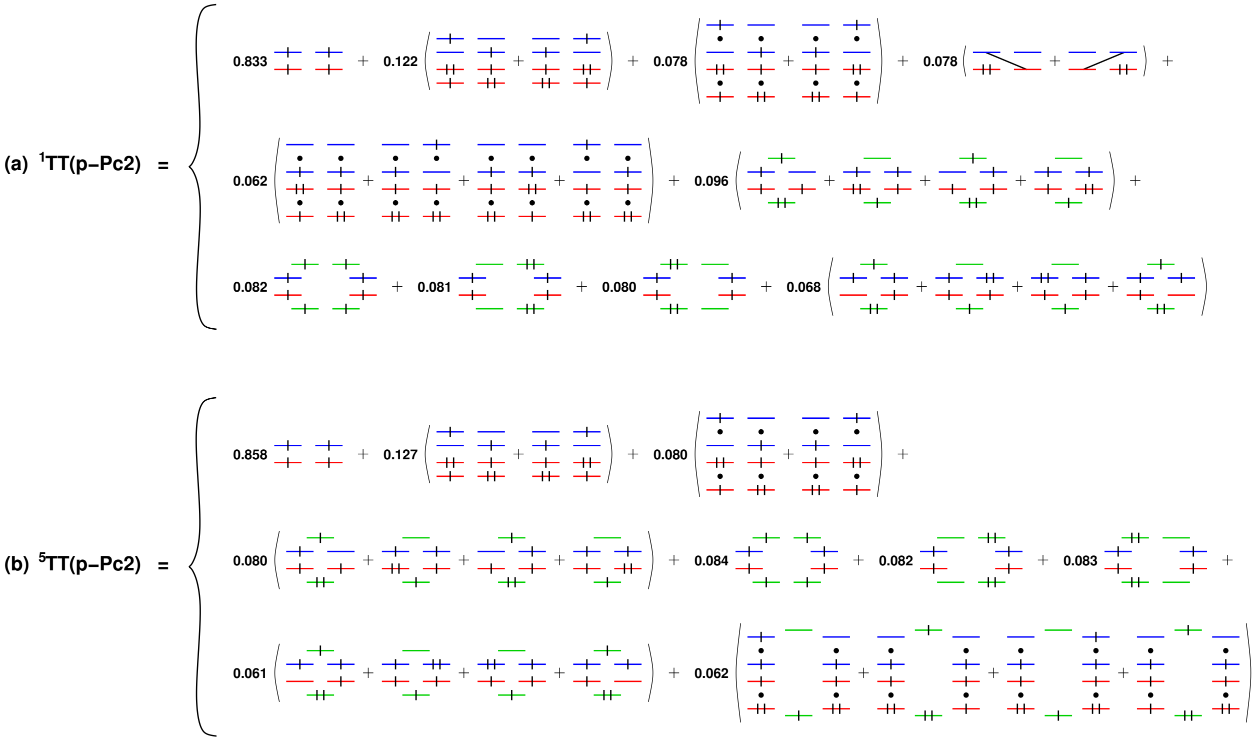


FIG. S2: Normalized correlated wavefunctions of (a) $^1$TT and (b) $^5$TT of *p*-Pc2. There is substantial difference between the wavefunctions. The dots represent intervening MOs completely filled or empty.

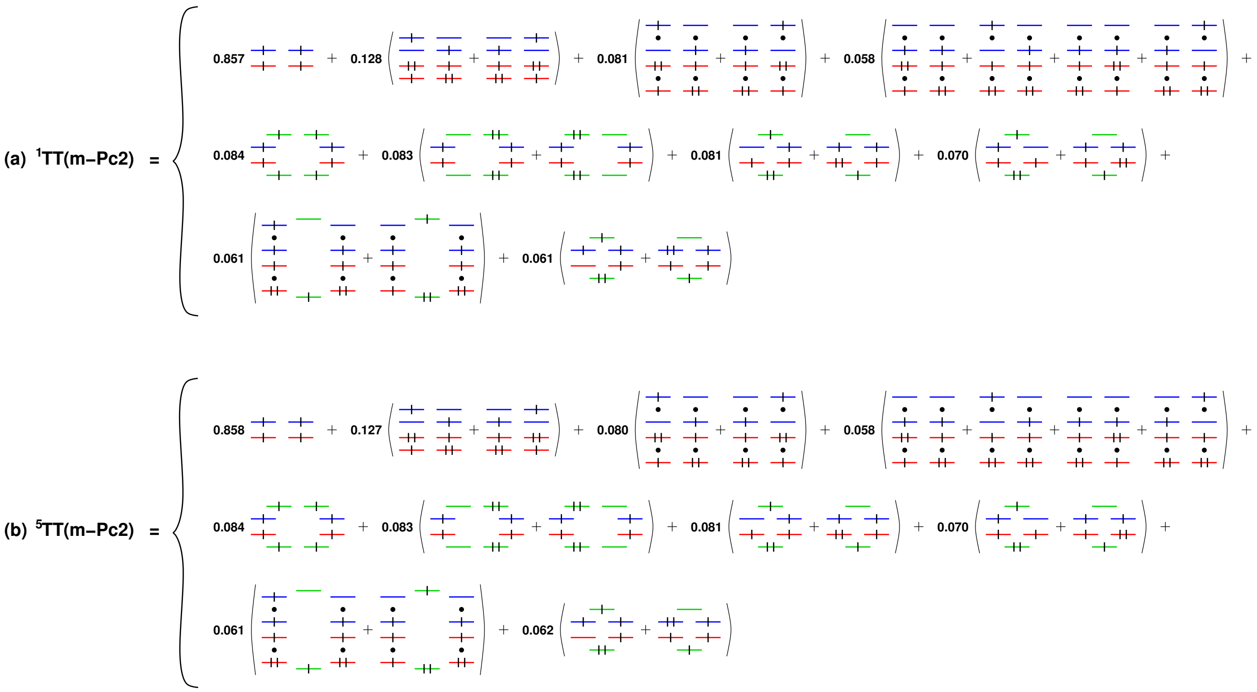


FIG. S3: Normalized correlated wavefunctions of (a) $^1$TT and (b) $^5$TT of *m*-Pc2. The two wavefunctions are completely identical, even as the individual configurations have $S_z = 0$ in (a) and $S_z = 2$ in (b).

## E. PENTACENE DIMERS INVESTIGATED EXPERIMENTALLY

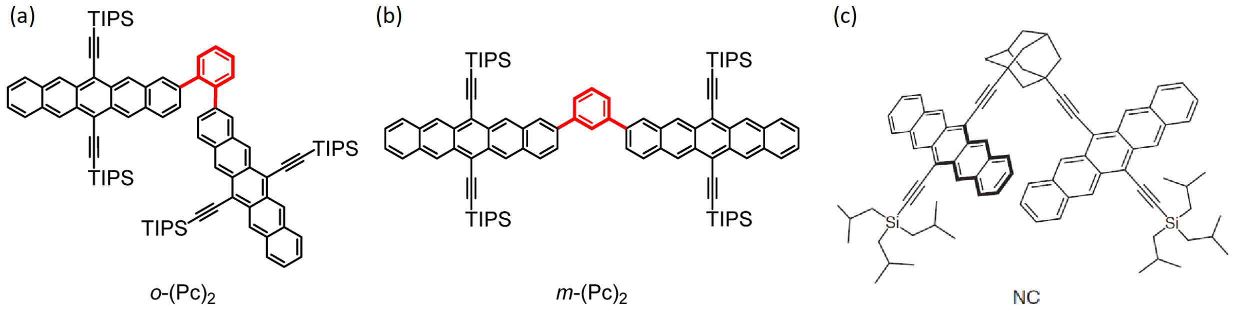


FIG. S4: (a, b) Ortho- and meta-linked (respectively) TIPS-pentacene dimers investigated by Sakai et al.[S1] (c) non-conjugated TIBS-pentacene dimer investigated by Basel, et al. [S2]

# References

**S1** Sakai, H.; Inaya, R.; Nagashima, H.; Nakamura, S.; Kobori, Y.; Tkachenko, N. V.; Hasobe, T. Multiexciton Dynamics Depending on Intramolecular Orientations in Pentacene Dimers: Recombination and Dissociation of Correlated Triplet Pairs. *J. Phys. Chem. Lett.*, **2018**, *9*, 3354-3360

**S2** Basel, B. S.; Zirzlmeier, J.; Hetzer, C.; Phelan, B. T.; Krzyaniak, M. D.; Reddy, S. R.; Coto, P. B.; Horwitz, N. E.; Young, R. M.; White, F. J., et al. Unified model for singlet fission within a non-conjugated covalent pentacene dimer. *Nat. Commun.*, **2017**, *8*, 15171
